# Supplementary material for: Tracking Counterfeit Cryptocurrency End-to-end
Source: arXiv:2011.02673 source file (2020-11-05)
Supplement: Supplementary file 1 [file appendix.tex]

\appendix

\setcounter{section}{0}

\begin{appendices}

\end{appendices}
